# Supplementary material for: PlenOctrees for Real-time Rendering of Neural Radiance Fields
Source: arXiv:2103.14024 source file (2021-08-17)
Supplement: Supplementary file 1 [file nerf_synth_table_correct.tex]

\begin{tabular}{@{}l c ccc c c}
\multicolumn{7}{c}{Synthetic NeRF Dataset \hspace{1em}\textfirst{best} \textsecond{second-best}}
\vspace{0.1em}\\
\toprule
 &  & PSNR $\uparrow$ & SSIM $\uparrow$ & LPIPS $\downarrow$ &  & FPS $\uparrow$ \\
\cmidrule{1-1} \cmidrule{3-5} \cmidrule{7-7}
NeRF (original) &  & 31.01 & 0.947 & 0.081 &  & 0.023 \\
NeRF &  & \cellthird 31.69 & \cellthird 0.953 & 0.068 &  & 0.045 \\
SRN &  & 22.26 & \fix{0.846} & 0.170 &  & \cellthird 0.909 \\
Neural Volumes &  & \fix{26.05} & \fix{0.893} & \fix{0.160} &  & \cellsecond 3.330 \\
NSVF &  & \cellfirst 31.75 & \cellsecond 0.953 & \cellfirst 0.047 &  & \fix{0.815} \\
AutoInt (8 sections) &  & 25.55 & 0.911 & 0.170 &  & 0.380 \\
\cmidrule{1-1} \cmidrule{3-5} \cmidrule{7-7}
\OurNeRF &  & 31.57 & 0.952 & \cellthird 0.063 &  & 0.051 \\
\orf{} from \OurNeRF &  & 31.02 & 0.951 & 0.066 &  & 167.68 \\
\orf{} after fine-tuning &  & \cellsecond 31.71 & \cellfirst 0.958 & \cellsecond 0.053 &  & \cellfirst 167.68 \\
\bottomrule
\end{tabular}
